# Supplementary material for: $\mathbb Z/2$-Godeaux surfaces
Source: arXiv:2009.12645 ancillary file (2026-04-28)
Supplement: Supplementary file 1 [file 1_TheAlgorithm_alpha_1_c_1.pdf]

## The Algorithm (case $\alpha_1$ with $c = 1$ )

This is an ancillary file for the paper  $\mathbb{Z}/2$ -Godeaux surfaces, by Eduardo Dias and Carlos Rito.

(Magma V2.25-5, JupyterLab 2.2.0)

Here we give the algorithm that allow us to compute the set of parameters such that the matrix  $\alpha$  satisfies the rank condition. Then we compute the equations of the étale double coverings of  $\mathbb{Z}/2$ -Godeaux surfaces for the case of the matrix  $\alpha_1$  with  $c = 1$  (see Theorem 4).

First we define a Magma function *LinElim* that will be used to solve our system of polynomial equations:

INPUT:  $f$  a sequence of polynomials,  $g$  a subset of  $f$ ,  $var$  a sequence of variables, and  $n \in \mathbb{N}$ .

PROCESS: It checks the elements of  $g$  one-by-one and whenever it finds one that is of the form  $r - h$  with  $r \in var$ ,  $h$  not depending on  $r$ , and containing at most  $n$  variables that are in  $var$ , it substitutes  $r$  by  $h$  in all elements of  $f, g$ . It also adds the pair  $[r, h]$  to a list that we call *dependencies*.

OUTPUT: The new list  $f$ , and the *dependencies*.

```
[1]: function LinElim(f,g,var,n)
    if g eq f then boo:=true;else boo:=false;end if;
    dependencies:=[];
    for v in var do
        for q in g do
            if v in Monomials(q) and
                q-Terms(q)[Position(Monomials(q),v)] eq Evaluate(q,v,0) and
                #{x:x in var | &or[IsDivisibleBy(m,x):m in Monomials(q)]} le n then
                // q = av+b
                b:=Evaluate(q,v,0); a:=(q-b) div v;
                Append(~dependencies,[v,-b/a]);
                f:={Evaluate(x,v,-b/a):x in f} diff {0};
                if boo then g:=f;else g:={Evaluate(x,v,-b/a):x in g} diff {0};end if;
                break;
            end if;
        end for;
    end for;
    return f,dependencies;
end function;
```

We can now start. We work on  $R[x, y_1, y_2, y_3, z_1, z_2, z_3, z_4, t]$  with  $R$  a polynomial ring with 394 variables (the parameters).

```
[2]: K:=Rationals();
R:=PolynomialRing(K,394);
A:=AffineSpace(R);
AssignNames(~R,["R." cat IntegerToString(i):i in [1..394]]);
RR<x,y1,y2,y3,z1,z2,z3,z4,t>:=PolynomialRing(R,[1,2,2,2,3,3,3,3,4]);
```

Recall that the involution  $\sigma$  is  $[-x, -y_1, y_2, -y_3, -z_1, -z_2, z_3, z_4, -t]$ . We compute sequences of monomials on  $[x, y_1, y_2, y_3]$  which are negative/positive for  $\sigma$ .

```
[3]: P<X,Y1,Y2,Y3>:=ProjectiveSpace(K,[1,2,2,2]);
h:=hom<CoordinateRing(P)->RR|[x,y1,y2,y3]>;
poly_m:=[h(m):m in Sections(LinearSystem(P,j)) |
          m eq -Evaluate(m,[-X,-Y1,Y2,-Y3])] :j in [1..8]];
poly_p:=[h(m):m in Sections(LinearSystem(P,j)) |
          m eq Evaluate(m,[-X,-Y1,Y2,-Y3])] :j in [1..8]];
```

We consider  $y_4 := dy_3$ , with  $d := R.23$ .

```
[4]: d:=R.23; y4:=d*y3;
```

We define the matrix  $\alpha$ , here denoted by  $M$ .

```
[5]: Q:=y1^2-y2^2-y3*y4;

G:=%+[R.i*poly_m[6][i]:i in [1..10]];

p1:=[y1*y2,y2*y3];
p2:=[x^2*y1,x^2*y3,y1*y2,y2*y3];
p3:=[x^4,x^2*y2,y2^2];
p4:=[x^4,y1*y3,y3^2];

q1:=%+[R.(10+i)*p1[i]:i in [1..2]];
q2:=%+[R.(12+i)*p2[i]:i in [1..4]];
q3:=%+[R.(16+i)*p3[i]:i in [1..3]];
q4:=%+[R.(19+i)*p4[i]:i in [1..3]];

M:=Matrix([
[x^2*G,x*q1,x*q2,x*q3,x*q4,Q],
[x*q1,y4,y1,y2,0,x],
[x*q2,y1,y3,x^2,y2,0],
[x*q3,y2,x^2,-y3,y1,0],
```

```
[x*q4,0,y2,y1,-y4,0],
[Q,x,0,0,0,0]
]);
```

Now we define a multi-sequence  $l$  such that the element  $l[i,j,k]$  is the polynomial  $l_{ij}^k$  that appears on the rank condition. Notice that these must be chosen with the right degree and  $\sigma$  sign.

```
[6]: l:=[[[RR|0:i in [1..6]]:j in [1..6]]:k in [1..6]];

B:=Adjoint(M);

Signs:=Matrix([[B[i,j] div Evaluate(B[i,j],[-x,-y1,y2,-y3,-z1,-z2,z3,z4,-t]):
               i in [1..6]]:j in [1..6]]);

ct:=23;
for k in [1..6] do for i in [2..6] do for j in [i..6] do
  deg:=Degree(B[i,j])-Degree(B[1,k]);
  sign:=Signs[i,j]/Signs[1,k];
  if sign eq -1 then
    l[i,j,k]:=&+[R.(h+ct)*poly_m[deg][h]:h in [1..#poly_m[deg]]];
    ct:=ct+#poly_m[deg];
  end if;
  if sign eq 1 then
    l[i,j,k]:=&+[R.(h+ct)*poly_p[deg][h]:h in [1..#poly_p[deg]]];
    ct:=ct+#poly_p[deg];
  end if;
end for;end for;end for;
```

The polynomials from the rank condition:

```
[7]: pol:=[RR[]];
for i in [2..6] do for j in [i..6] do
  Append(~pol,B[i,j]-&+[l[i,j,k]*B[1,k]:k in [1..6]]);
end for;end for;
```

And their coefficients:

```
[8]: f:=&join[Seqset(Coefficients(q)):q in pol];
f:=SetToIndexedSet(f);
```

Our goal is to compute the parameters such that the polynomials in  $f$  vanish.

We now use the Magma function `LinElim` defined above to solve the system of equations  $f = 0$ . We expect to eliminate all variables except  $d$  and some of the  $g_i$  and  $b_j$  (which are the first 23 variables of the ring  $R$ ). So, we use the function for the remaining 371 variables. After this we see that there is a set  $g \subset f$  of polynomials containing only variables  $d, g_i$  or  $b_j$ , and such that some of these variables can also be eliminated. So we run `LinElim(f, g, var, n)` now with  $var = [g_1, \dots, g_{10}, b_1, \dots, b_{12}]$ .

This process is much more efficient if we do it for  $n = 1$ , then repeat for  $n = 2$ , etc. The system is solved when the output  $f$  is empty. We do it and it ends after 9 iterations.

```
[9]: dependencies:=[];
for n in [1..9] do
  f,dep:=LinElim(f,f,[R.i:i in [23+1..394]],n);
  dependencies:=dependencies cat dep;
  g:={@ @};
  for q in f do
    if &and[IsDivisibleBy(m,x) eq false: x in [R.i:i in [23+1..394]],
      m in Monomials(q)] then
      Include(~g,q);
    end if;
  end for;
  f,dep:=LinElim(f,g,[R.i:i in [1..22]],22);
  dependencies:=dependencies cat dep;
end for;
#f;
```

0

We write the *dependencies* depending on the minimum possible number of variables.

```
[10]: for i in [#dependencies..1 by -1] do for j in [i-1..1 by -1] do
  dependencies[j]:=[dependencies[j][1],
    Evaluate(dependencies[j][2],dependencies[i][1],dependencies[i][2])];
end for;end for;
```

And we check which are the variables in  $\{d, g_1, \dots, g_{10}, b_1, \dots, b_{12}\}$  that remain in our system.

```
[11]: &join[{x:x in [R.i:i in [1..23]] |
  &or[IsDivisibleBy(m,x):m in Monomials(q[2])]}:q in dependencies];
```

```
{
R.16,
R.21,
R.9,
R.18,
R.22,
R.12,
R.19,
```

```
R.15,
R.23
}
```

We can now compute the matrix  $\alpha = M$ , by evaluating its polynomial coefficients at the *dependencies*.

```
[12]: for i in [1..6] do for j in [1..6] do
      if IsCoercible(Integers(),M[i,j]) eq false then
        for q in dependencies do
          cf:=Coefficients(M[i,j]);mon:=Monomials(M[i,j]);
          cf:=[Evaluate(R!x,q[1],q[2]):x in cf];
          M[i,j]:=&+[cf[k]*mon[k]:k in [1..#cf]];
        end for;
      end if;
    end for;end for;
```

We do the same for the  $l_{ij}^k$ .

```
[13]: for k in [1..6] do for i in [2..6] do for j in [i..6] do
      for q in dependencies do
        if l[i,j,k] ne 0 then
          cf:=Coefficients(l[i,j,k]);mon:=Monomials(l[i,j,k]);
          cf:=[Evaluate(R!x,q[1],q[2]):x in cf];
          l[i,j,k]:=&+[cf[i]*mon[i]:i in [1..#cf]];
        end if;
      end for;
    end for;end for;end for;
```

We can finally compute the equations given by Section 2 (6), on the variables  $x, y_1, y_2, y_3, z_1, z_2, z_3, z_4, t$ .

```
[14]: v:=[1,z1,z2,z3,z4,t];
Eqs:=[];
for i in [2..6] do for j in [i..6] do
  Append(~Eqs, -v[i]*v[j]+&+[l[i,j,k]*v[k]:k in [1..6]] );
end for;end for;

Eqs:=Eqs cat RowSequence(Transpose(M*Matrix(6,1,[1,z1,z2,z3,z4,t]))) [1];
```

We save these equations in a file.

```
[15]: AssignNames(~R,["g" cat IntegerToString(i):i in [1..10]] cat
      ["b" cat IntegerToString(i):i in [1..12]] cat
```

```

["d"] cat
["R." cat IntegerToString(i):i in [24..394]]);
PrintFile("2_EqsNotYetFinal_alpha_1_c_1.txt","Eqs:=" cat Sprint(Eqs) cat ";" :
→Overwrite:=true);

```

The equations of degree  $\leq 5$  depend only on some of the first 23 variables of the ring  $R$  (which are  $d$  and the  $g_i$  and  $b_j$ ). But this is not true for the other equations. We show that the coefficients of the  $R.i$  with  $i > 23$  are contained in the ideal generated by the equations of degree  $\leq 5$  (see the arXiv ancillary file 3\_RemovingTheRi\_alpha\_1\_c\_1.txt), so we can consider  $R.i = 0$  for  $i > 23$ .

The final equations are then:

```

[16]: for i in [1..#Eqs] do
      cf:=Coefficients(Eqs[i]);
      mon:=Monomials(Eqs[i]);
      cf:=[Evaluate(q,[R.i:i in [1..23]] cat [0:i in [24..394]]):q in cf];
      Eqs[i]:=&+[cf[i]*mon[i]:i in [1..#cf]];
    end for;

```

We save them in a file:

```

[17]: PrintFile("4_TheEquations_alpha_1_c_1.txt","M:=" cat Sprint(RowSequence(M)) cat
→";":Overwrite:=true);
PrintFile("4_TheEquations_alpha_1_c_1.txt","Eqs:=" cat Sprint(Eqs) cat ";" );

```
